# Supplementary material for: Bridging Human Evaluation to Infrared and Visible Image Fusion
Source: arXiv:2603.03871 source file (2026-03-04)
Supplement: Supplementary file 1 [file X_suppl.tex]

\clearpage
\setcounter{page}{1}
\maketitlesupplementary

% \section{Overview}  

\section{Human Feedback Dataset Construction}
\label{sec:rationale}

\subsection{Data Cleaning Pipeline}
\noindent To construct a human feedback IVIF dataset to support the modeling and evaluation of perceptual consistency, we collected 31,769 infrared-visible image pairs from 8 benchmark datasets (FMB~\cite{liu2023multi}, LLVIP~\cite{jia2021llvip}, M\(^{3}\)FD~\cite{liu2022target}, MFNet~\cite{ha2017mfnet}, RoadScene~\cite{xu2020u2fusion}, SMOD~\cite{chen2024amfd}, TNO
% ~\cite{toet2017tno}
, and VIFB). Since the dataset contained a large number of duplicate scenes, we used the CLIP model for data cleaning

Given that the CLIP model is primarily pre-trained on visible domain images, we employ the CLIP ViT-B/32 model to perform semantic analysis on visible images. We first extract CLIP feature vectors for all visible images and apply $L2$ normalization. Through extensive experiments, we determined an optimal cosine similarity threshold of 0.85, which effectively balances diversity preservation and redundancy removal—retaining 1,257 representative images.
For each similar scene cluster identified through CLIP analysis, we implement a selection process that evaluates images based on multiple quality dimensions: visual quality metrics (sharpness and contrast), resolution, and information content (using file size as a proxy indicator). The selection process employs a weighted scoring system, with visual quality as the most important factor (50\%), followed by resolution (30\%), and information content contributing the remaining 20\% weight. This approach ensures that the highest quality representative image is retained from each semantic cluster, ultimately filtering down to 900 representative visible-light images paired with their corresponding infrared images. Further expert screening was conducted on the CLIP-cleaned data, ultimately yielding 850 pairs of high-quality images.

\subsection{Large Models and Human Feedback}
\noindent We first invited four senior experts with over five years of research experience in infrared and visible image fusion (IVIF) to provide refined scores for 100 data triplets and annotate artifact regions using center coordinates and radii, yielding a high-quality seed dataset. Each triplet comprises a visible image, an infrared image, and a fused image, requiring approximately five minutes for annotation. The total annotation time per annotator was approximately 500 minutes (about 8 hours). The detailed dataset annotation guidelines are shown in ~\cref{tab:annotation_guidelines}.

\begin{listing}[htbp]
\caption{Example JSON output from GPT-4o}
\label{lst:json_output}
\hrule\vspace{4pt}
\begin{minted}[
    frame=none,
    baselinestretch=1.2,
    fontsize=\small,
    style=bw              % 添加这一行，使用黑白样式
]{json}
{
  "scores": {
    "Thermal Retention": 4,
    "Texture Preservation": 3,
    "Artifacts": 2,
    "Sharpness": 3,
    "Overall Score": 3
  },
  "shapes": [
    {
      "label": "Artifacts",
      "points": [[390, 420], [430, 420]],
      "shape_type": "circle"
    },
    {
      "label": "Artifacts",
      "points": [[250, 170], [290, 170]],
      "shape_type": "circle"
    }
  ]
}
\end{minted}
\vspace{4pt}\hrule
\end{listing}

\begin{table*}[t] 
\centering 
\caption{Annotation Guidelines for Human Feedback Dataset} 
\label{tab:annotation_guidelines} 
\begin{tabular}{
    >{\centering\arraybackslash}m{3.5cm}
    >{\centering\arraybackslash}m{4cm}
    p{8.5cm}
} 
\toprule 
\textbf{Category} & 
\textbf{Item} & 
\multicolumn{1}{c}{\textbf{Description and Details}} \\ 
\midrule 
\multirow{16}{3cm}{\centering\textbf{Evaluation Criteria} \\ (1-5 points)} & 
\textbf{1. Thermal Retention} & 
Quantifies preservation accuracy of heat sources' intensity, distribution, and spatial positioning in fused images. \\ 
\cmidrule(lr){3-3} 
& & 
\textbullet~High-heat signatures (e.g., humans/vehicles) from infrared imagery \\ 
& & 
\textbullet~Structural thermal patterns unique to infrared imaging in low-light conditions (e.g., buildings) \\ 
& & 
\textbullet~Environmental texture retention \\ 
\cmidrule(lr){2-3} 
& 
\textbf{2. Texture Preservation} & 
Measures the fidelity of visible-light details and textures in fused results. \\ 
\cmidrule(lr){3-3} 
& & 
\textbullet~Surface/edge clarity of objects \\ 
& & 
\textbullet~Resistance to visible information occlusion by infrared data \\ 
& & 
\textbullet~Structural integrity of fine-grained patterns \\ 
\cmidrule(lr){2-3} 
& 
\textbf{3. Artifacts} & 
Identifies unnatural distortions including: \\ 
\cmidrule(lr){3-3} 
& & 
\textbullet~Bright spots \\ 
& & 
\textbullet~Ghost shadows \\ 
& & 
\textbullet~Physically implausible anomalies \\ 
\cmidrule(lr){2-3} 
& 
\textbf{4. Sharpness} & 
Evaluates overall visual coherence through: \\ 
\cmidrule(lr){3-3} 
& & 
\textbullet~Edge definition precision \\ 
& & 
\textbullet~Detail completeness \\ 
& & 
\textbullet~Perceptual clarity \\ 
\midrule 
\textbf{Heatmap Annotation} & 
\textbf{1. Artifact Marking} & 
\textbf{Label:} Artifacts \\ 
\cmidrule(lr){3-3} 
& & 
\textbf{Method:} Encircle anomalous regions using circular annotations (center coordinates + radius) \\ 
\cmidrule(lr){3-3} 
& & 
\textbf{Note:} For elongated artifacts, approximate coverage with minimally sized circles \\ 
\bottomrule 
\end{tabular} 
\end{table*}

\begin{figure*}[t]
    \centering
    \includegraphics[width=1\linewidth]{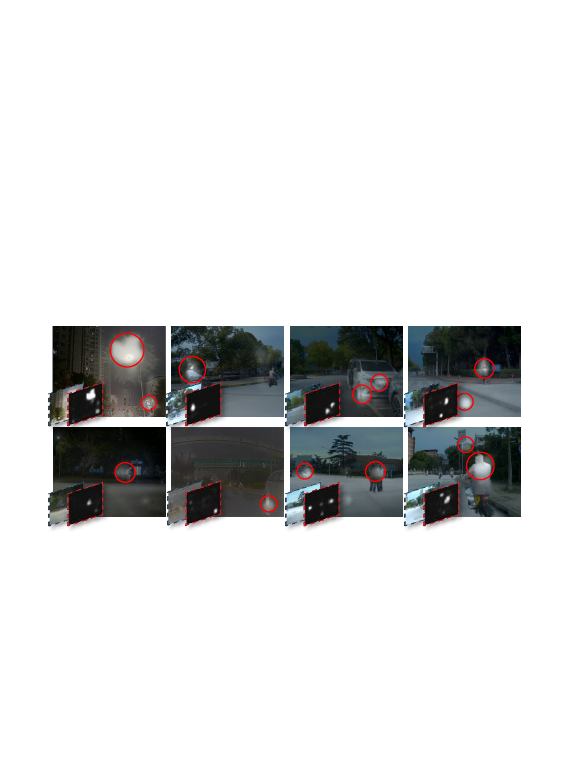}
    \caption{Heatmap visualization generated by the reward model on fused images, with artifact regions highlighted by red circles.}
    \label{fig:heat}
    \vspace{-3mm}
\end{figure*}  

Using the obtained seed dataset, we aligned the GPT-4o model (specifically version gpt-4o-2024-08-06 accessed via the OpenAI API) with expert preferences. This alignment is a prompt-driven process achieved through In-Context Learning. When constructing the input context, we embedded the evaluation guidelines from ~\cref{tab:annotation_guidelines} as system instructions into each query to guide the model in understanding the specific meanings and scoring criteria for each evaluation dimension. 
During this alignment phase, GPT-4o receives visible, infrared, and fused image triplets as inputs to perform systematic multi-dimensional evaluations across thermal retention, texture preservation, artifacts, and sharpness. To ensure the model's outputs strictly adhere to human expert judgment, we iteratively optimized the system prompts and selected effective few-shot exemplars from the seed dataset. 
By minimizing the discrepancy between the model outputs and the expert labels in the seed dataset, we determined the optimal prompt configuration and exemplar combination. This discrepancy is measured by a composite error metric. The first component is the scoring discrepancy, derived by computing the normalized Mean Squared Error (MSE) between the model's predicted scores and ground-truth expert values across the four evaluation dimensions. The second component is the artifact heatmap discrepancy, obtained from the Binary Cross-Entropy (BCE) between the generated artifact circular regions and the expert-annotated heatmaps. 
% The total evaluation discrepancy function is defined as:
% \begin{equation}
% \mathcal{E}_{\text {total }} = \lambda_1 \mathcal{L}_{\mathrm{MSE}} + \lambda_2 \mathcal{L}_{\mathrm{BCE}},
% \end{equation}
% where $\lambda_1 = 0.6$ and $\lambda_2 = 0.4$.

The JSON format output by the GPT-4o model contains four fundamental quality scores and artifact heatmap annotations. Each artifact region is defined by two coordinate points: the first point specifies the circle center, and the second point lies on the circumference; together, they determine the precise location and extent of the artifact marking.
The example JSON output is shown in ~\cref{lst:json_output}.

% After fine-tuning was completed, 
Then, we used the GPT-4o model to automatically annotate all 9,350 fused images. To ensure the accuracy of the automated annotations, we established a rigorous human quality control process. We invited 5 researchers with at least 3 years of research experience in the IVIF field. The review work was divided into two stages:

\textbf{Sampling Inspection (15 hours).} Each reviewing expert was randomly assigned 200 annotated images for detailed inspection, achieving a total review coverage rate of $10.7\%$ (1,000/9,350). Experts needed to evaluate: (1) whether the scores conformed to the evaluation guideline standards; (2) whether the artifact region annotations were complete and accurate; (3) whether there were systematic biases or error patterns. Through this stage, we identified the following main issues: $8\%$ of images had scoring deviations; $12\%$ of images had incomplete artifact annotations, missing artifacts in certain regions.

\textbf{Comprehensive Correction and Consistency Calibration (150 hours).} Based on the problem patterns identified in the first stage, the review team conducted a systematic review of all 9,350 images. The specific work included: (1) Scoring standard calibration: for images with scoring deviations, experts re-evaluated the scores according to the evaluation guidelines to ensure scoring consistency; (2) Artifact annotation correction: for missed artifact regions, experts supplemented annotations, particularly targeting small artifacts and blurry edge regions, and removed false artifact annotations by comparing the infrared and visible source images; (3) Extreme case discussion: for images where the 5 experts disagreed ($3\%$), collective discussions were organized to reach consensus.

Through this rigorous quality control process, the annotation quality of the final dataset was significantly improved. The final human feedback IVIF dataset was used to train the fusion-oriented reward model.

\section{Heatmap Visualization}
% \noindent To intuitively demonstrate the artifact identification capability of our trained fusion-oriented reward model, we conducted heatmap visualization analysis on images generated by different fusion methods, as shown in ~\cref{fig:heat}. The highlighted regions (red/warm colors) in the heatmaps indicate artifact or quality degradation areas identified by the model, while low-intensity regions (blue/cool colors) represent normal areas with good quality. It can be observed that our reward model accurately localizes various types of artifacts in fused images, including bright spots, ghosting, and structural distortions. This visualization validates the effectiveness of the reward model in quantifying human perceptual preferences, providing reliable guidance signals for subsequent RLHF optimization.
\noindent To intuitively demonstrate the artifact identification capability of our trained fusion-oriented reward model, we conducted heatmap visualization analysis on images generated by different fusion methods, as shown in ~\cref{fig:heat}. The red circles highlight artifact regions identified by the model, including bright spots, ghosting, and structural distortions. This visualization validates the effectiveness of the reward model in quantifying human perceptual preferences, providing reliable guidance signals for subsequent RLHF optimization.

\section{Policy Optimization Strategy Ablation}
\noindent To validate the effectiveness of our proposed optimization strategy, we compare it with Proximal Policy Optimization (PPO) and Direct Preference Optimization (DPO).
% \noindent To validate the effectiveness of our proposed optimization strategy, we compare it with Proximal Policy Optimization (PPO)~\cite{schulman2017proximal} and Direct Preference Optimization (DPO)~\cite{rafailov2023direct}.

For PPO, we implemented a value network as the critical model with a value loss coefficient of 0.5, using standard hyperparameters including a clipping parameter $\epsilon$ of 0.2 and GAE parameter $\lambda$ of 0.95. The KL penalty coefficient $\beta$ was set to 0.01, with early stopping when KL divergence exceeded 0.015 to prevent excessive policy deviation. For DPO, we followed the official formulation with $\beta=0.1$, using the Bradley-Terry model for preference learning while keeping the reference model fixed during training, which is consistent with the standard DPO implementation.
